# Supplementary material for: On the Relationship Between Interpretability and Explainability in Machine Learning
Source: arXiv:2311.11491 source file (2024-04-25)
Supplement: Supplementary file 1 [file supplementary.tex]

\subsection{The Complete BGN Algorithm}\label{sec:bgn_algos}

\begin{algorithm}[h]
	\caption{The complete BGN algorithm}
	\begin{algorithmic}[1]\label{algo:bgn_general}
	\STATE \textbf{Input} : $S = \{(\xbf_1,y_1),\dots,(\xbf_m,y_m)\}$, $\ybf \in \mathbb{R}$, $\xbf\in\mathbb{R}^d$, a dataset
	\STATE Set $\{\mathbf{x}_i^{(1)}\}_{i=1}^m = \{\mathbf{x}_i\}_{i=1}^m$
	\STATE \textbf{For} $z = 1,\dots,l-1$ :
    \STATE $\quad$ Set $\mathbf{r}^{(1)} = \ybf$, $t=0$, $b_{z+1} = 0$, $\Wbf_{z} = \textbf{0}_{d_{z-1}\times d_{z}}$, $\bbf_{z} = \textbf{0}_{d_{z}}$
	\STATE $\quad$ \textbf{While} stopping criterion is not met:
	\STATE $\quad\quad$ $t = t + 1$
    \STATE $\qquad$ $\wbf_{z,t} = \textup{LassoRegression}(S^{(z,t)})$,
	\quad where $S^{(z,t)}= \{(\xbf_1^{(z)},r_1^{(t)}),\dots,(\xbf_m^{(z)},r_m^{(t)})\}$
    \STATE $\qquad$ $b_{z,t} = {\argmin}_b\ \left( \frac{|\mathbf{r}^{(z,t)}_{-1}|}{m}\textup{Var}\left(\mathbf{r}^{(z,t)}_{-1}\right)+\frac{|\mathbf{r}^{(z,t)}_{+1}|}{m}\textup{Var}\left(\mathbf{r}^{(z,t)}_{+1}\right)\right)$ \\
    \STATE $\qquad\qquad\qquad\quad$ with $\mathbf{r}^{(z,t)}_{\pm1}$ given by Eq.~\eqref{eq:ypm}, but with $\{\mathbf{x}_i^{(t)}\}_{i=1}^m$ instead of $\{\mathbf{x}_i\}_{i=1}^m$
	\STATE  $\qquad$ $\rho_\pm^{(z,t)} = \dfrac{\sum_{i:\sgn\left(\xbf_i^{(z)}\cdot\mathbf{w}_{z,t}+b_{z,t}\right)=\pm1} r_i^{(t)}}{\sum_{i:\sgn\left(\xbf_i^{(z)}\cdot\mathbf{w}_{z,t}+b_{z,t}\right)=\pm1} 1}$
    %\STATE $\qquad\quad\qquad\qquad\qquad\qquad\qquad\qquad\qquad$ with $\rho_{j\pm}^{(z,t;p)} = \frac{\sum_{i:\sgn(\xbf_i^{(z)}\cdot\mathbf{w}_{z,p}+b_{z,p})=\pm1} r_{i,j}^{(t)}}{\sum_{i:\sgn(\xbf_i^{(z)}\cdot\mathbf{w}_{z,p}+b_{z,p})=\pm1} 1}$
	\STATE $\qquad$ $w_{z+1,t} = \frac{1}{2}\left(\rho_+^{(z,t)}-\rho_-^{(z,t)}\right); \quad  b_{z+1,t} = \frac{1}{2}\left(\rho_+^{(z,t)}+\rho_-^{(z,t)}\right)$
    \STATE $\quad\quad$ $r^{(t+1)}_{i}=r^{(t)}_{i} - w_{z+1,t}\ \sgn(\mathbf{w}_{z,t}\cdot\mathbf{x}_i^{(z)}+b_{z,t}) - b_{z+1,t}$\ \ $\forall i \in \{1,\dots,m\}$
	\STATE $\quad\quad$ $p^*=1$
	\STATE $\quad\quad$ \textbf{While} $p^* < t$:
	\STATE $\quad\quad\quad$ $p$ = random.int($1,t$)
    \STATE $\qquad\quad$ $\delta$ = $\overline{\mathbf{r}^{(p)}}$
	\STATE $\qquad\quad$ $\gamma$ = ($\wbf_{z,p}$, $b_{z,p}$, $w_{z+1,p}$, $b_{z+1,p}$, $\mathbf{r}^{(p)}$) \hfill [Save values]
    \STATE $\quad\quad\quad$ $r^{(p)}_{i}=r^{(p)}_{i} + w_{z+1,p}\ \sgn(\mathbf{w}_{z,p}\cdot\mathbf{x}_i^{(z)}+b_{z,p}) + b_{z+1,p}$\ \ $\forall i \in \{1,\dots,m\}$
    \STATE $\qquad\quad$ Do steps 8-12, with $t:=p$
	\STATE $\quad\quad\quad$ $r^{(p)}_{i}=r^{(p)}_{i} - w_{z+1,p}\ \sgn(\mathbf{w}_{z,p}\cdot\mathbf{x}_i^{(z)}+b_{z,p}) - b_{z+1,p}$\ \ $\forall i \in \{1,\dots,m\}$
    \STATE $\qquad\quad$ \textbf{If} $\overline{\mathbf{r}^{(p)}} > \delta$
    \STATE $\qquad\qquad$ ($\wbf_{z,p}$, $b_{z,p}$, $w_{z+1,p}$, $b_{z+1,p}$, $\mathbf{r}^{(p)}$) = $\gamma$ \hfill [Restore values]
    \STATE $\qquad\quad$ $p^* = p^* + 1$
	\STATE $\quad$ $\mathbf{x}_i^{(z+1)} = (L_{z}\circ\dots\circ L_1)(\mathbf{x}_i) \forall i \in \{1,\dots,m\}$
	\STATE \textbf{Output} : $BGN_T(\xbf)$ = $\sum_{t=1}^T \mathbf{c}_t\ (L_{l-1}\circ\dots\circ L_1)(\mathbf{x})+\mathbf{d}_t$
	\end{algorithmic} 
\end{algorithm}

\subsection{Details about the numerical experiments}\label{subsec:num}

\begin{table}[t]
    \centering
    \caption{Datasets overview (F = Floats, I = Integers)}
    \label{tab:algo_overview}
    \setlength{\tabcolsep}{4pt}
    {\small
    \begin{tabular}{lllllllll}
    \toprule
    \# & Dataset & Full name & Taken from & Source & $d$ & Type of $\mathbf{x}$ & $m$\\
    \midrule
    1 & bike hour & Bike sharing dataset & UCI Repo. & \cite{bike} & 16 & F/I & 17 389 \\
%    2 & carbon & Carbon nanotubes & UCI Repo. & \cite{carbon1} & 3 & 5 & F & 10 721\\
    2 & diabete & Diabetes & SKLearn & \cite{efron2004least} & 10 & F/I & 442 \\
    3 & housing & California housing & SKLearn & \cite{HARRISON197881} & 8 & F & 20 640 \\
    4 & hung pox & Hungarian chickenpox cases & UCI Repo. & \cite{rozemberczki2021chickenpox} & 20 & F & 521 \\
    5 & ist. stock & Istanbul stock exchange (USD) & UCI Repo. & \cite{Akbilgic2014ANH} & 8 & F & 536 \\
    6 & parking & Parking Birmingham & UCI Repo. & \cite{10.1007/978-3-319-59513-9_11} & 4 & F & 35 717 \\
    7 & power p. & Combined cycle power plant & UCI Repo. & \cite{TUFEKCI2014126,HeysemKayaLocalAG} & 4 & F & 9568 \\
    % 9 & solar flare & Solar flare & UCI Repo. & \cite{Dua:2019} & 3 & 10 & C & 1389 \\
    % 10 & stock portfolio & Stock portfolio performance & UCI Repo. & \cite{portfolio} & 6 & 6 & F & 315 \\
    % 11 & turbine & Gas Turbine CO and NOx & UCI Repo. & \cite{turbine} & 2 & 10 & F & 36 733 \\ \addlinespace[-1.5mm]
    % & & emission data set & & & & & & \\
    \bottomrule
    \end{tabular}
    }
\end{table}

\begin{table}[t]
    \centering
    \caption{Benchmarks overview}
    \label{tab:methods_overview}
    \setlength{\tabcolsep}{3pt}
    {\small
    \begin{tabular}{l||c|ccccc}
    \cline{1-7}
    Algorithm & BGN & BC & BNN$^*$ & BNN+ & Bi-real net$^*$ & QN\\
    \cline{1-7}
    Weights & $\mathbb{R}$ & $\{-1,+1\}$ & $\mathbb{R}$ & $\mathbb{R}$ & $\mathbb{R}$ & $\mathbb{R}$\\
    Activations output & $\{-1,+1\}$ & $\mathbb{R}$ & $\{-1,+1\}$ & $\{0,1\}$ & $\{-1,+1\}$ & $\{0,1\}$\\
    Uses batch norm & False & True & True & True & True & True\\
    Uses regularization & False & False & False & True & False & False\\
    \cline{1-7}
    \end{tabular}
    }
\end{table}

\paragraph{Hyperparameters selected on the validation set}
\begin{itemize}
    \item Number of hidden layers : 1,2,3
    \item Width: 100, 500, 1000
    \item Learning rates: 0.1, 0.01, 0.001
    \item Regularization type (BNN+): $L_1$, $L_2$ ($10^{-6}$, $10^{-7}$)
    \item $\beta$ values (BNN+): 1, 2, 5
    \item $T_{\textup{Start}}$ values (QN): 5, 10, 20 (while $T_{\textup{At epoch n}}$ = $T_{\textup{Start}} * n$)
\end{itemize}

\paragraph{Fixed hyperparameters}
\begin{itemize}
    \item Initialization: Kaiming uniform  \cite{DBLP:conf/iccv/HeZRS15}
    \item Batch size: 512 for big datasets (over 9000 examples) and 64 for small ones (see \autoref{tab:algo_overview})
    \item Maximum number of epochs: 200 (early stop: 20)
%    \item Loss function: Mean squared error (MSE)
    \item Optimization algorithm: Adam \cite{DBLP:journals/corr/KingmaB14},\\ with $\epsilon = 0.001, \rho_1 = 0.9, \rho_2 = 0.999, \delta = 10^{-8}, 
    \lambda=0 $
    % \begin{itemize}
    %     \item $\epsilon$ = 0.001
    %     \item $\rho_1 = 0.9, \rho_2 = 0.999$
    %     \item $\delta = 1e-8$
    %     \item $\lambda$ = 0
    % \end{itemize}
    \item Learning rate decay: plateau (patience: 5)
\end{itemize}

%The test set was always composed of 25\% of the total dataset (if the train-test separation isn't inherent to the problem), while the validation set was 20\% of the remaining data.\\

\subsection{Extended details on the interpretability and explainability experiments}\label{sec:int-expl}

The experiments were conducted on five random seeds, for BGN as well as for the regression tree. As for the tree, the following hyperparameter choices were considered (with the retained set of hyperparameter being bolded): maximum number of features (\textit{d}) considered at each split: \textbf{d}, $\sqrt{d}$, $log_2(d)$; criterion: \textbf{squared error}, Friedman MSE, absolute error, poisson; the strategies used to choose the split at each node: random, \textbf{best}.

\begin{table}[t]
\caption{Comparison between trees of depth 3, 4 and 5 and 1-BANNs having correspondingly similar mean test MSE on the \textit{housing} dataset. We present the tree depth and the 1-BANN width ($d_1$) as a metric for comparing their complexity, as well as the number of considered features of the models ($d_0^*$).}
\centering
\setlength{\tabcolsep}{2pt}
\begin{tabular}{|c c|cc|} 
 \hline
 Model & Test MSE & (Depth, $d_1$) & $d_0^*$ \\
 \hline\hline
 1-BANN & 0.6358 & 5 & 3 \\
 Tree & 0.6413 & 3 & 3 \\ 
 \hline
 1-BANN & 0.5849 & 7 & 4 \\
 Tree & 0.5779 & 4 & 5 \\
 \hline
 1-BANN & 0.5020 & 8 & 5 \\
 Tree & 0.5291 & 5 & 6 \\
 \hline
\end{tabular}
\label{tab:perf-compl}
\end{table}

\autoref{tab:perf-compl} shows how, on the \textit{housing} dataset, as trees become deeper, thus exponentially more powerful and complex, BGN only has to yield 1-BANNs having a few more hidden neurons in order to keep up with the gains in predictive performances. We see that the required width of the 1-BANNs grows almost linearly, and while the depth of the tree has a huge impact on its interpretability, the width of the 1-BANN has a relationship to its interpretability that it way less important (as analyzed in \autoref{subsec:intexp}).
